# Supplementary material for: Diffusion Transformers with Representation Autoencoders
Source: arXiv:2510.11690 source file (2025-10-13)
Supplement: Supplementary file 1 [file implementation_details.tex]

\section{Implementation Details}

\subsection{Sequence and Patch Configuration}
We explore different configurations for handling image sequences and patches.
\subsubsection{High-Resolution Generation (512x512)}
We investigate two methods for 512x512 generation: directly increasing the number of tokens by 4x, and using the decoder to upsample the latent representation from a smaller token set.
\subsubsection{Patch Size Variation}
We experiment with different encoder patch sizes, such as 8 and 32, and analyze their impact on generation. We also explore techniques like token unshuffling.
